# Supplementary material for: Probabilistic Forecasting of Irregular Time Series via Conditional Flows
Source: arXiv:2402.06293 source file (2025-01-13)
Supplement: Supplementary file 1 [file appendix-cnf-vs-umnn.tex]

\section{Unconstrained monotonic neural networks are just continuous normalizing flows}
\label{app:umnn-vs-cnf}
Any unconstrained monotonic neural network \citep{Wehenkel2019.Unconstrained}
can equivalently be written as a standard continuous normalizing flow.
To make our deduction of the \act activation function in section~\label{sec:act}
slightly more streamlined, we therefore have presented 
unconstrained monotonic neural network as continuous normalizing flows
from the beginning.

Lemma. Any UMNN function $a$ defined by
\begin{align*}
    a^{\text{UMNN}}(x) & := \int_0^x g(\tau, a(\tau)) d\tau + b
\end{align*}
one can get as a continuous normalizing flow for a suitable scalar field $\tilde g$:
\begin{align*}
     a^{\text{CNF}}(x) & := v(1)
 \quad \text{with } v : \R\rightarrow\R
   \text{ being the solution of }
   \frac{\partial v}{\partial\tau} = \tilde g(\tau, v(\tau)),
        \quad   v(0)  := x
\end{align*}

Proof.
Choose
\begin{align*}
\tilde g(\tau, v):= g(\tau x, v(\tau x)) x + b - x
\end{align*}

The solution of the continuous normalizing flow is
\begin{align*}
     a^{\text{CNF}}(x) & = v(x) = \int_0^1 \tilde g(\tau, v(\tau)) \,d\tau + x
    \\ & = \int_0^1  ( g(\tau x, v(\tau x)) x + b  - x)     \, d\tau + x
    \\ & = \int_0^1  g(\tau x, v(\tau x)) x \,d\tau + b
    \\ & = \int_0^x  g(\frac{\tau}{x} x, v(\frac{\tau}{x} x)) \,d\tau + b
    \\ & = \int_0^x  g(\tau, v(\tau)) \,d\tau + b
      = a^{\text{UMNN}}(x)         
\end{align*}

%%% Local Variables:
%%% mode: latex
%%% TeX-master: "profiti-lst"
%%% End:
